# Supplementary material for: Gravitational lenses in arbitrary space-times
Source: arXiv:2011.04440 source file (2022-05-09)

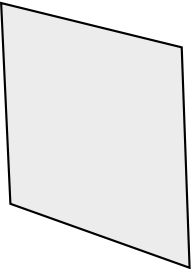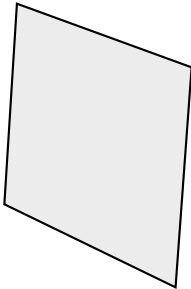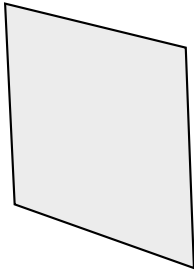

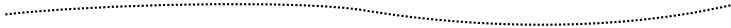

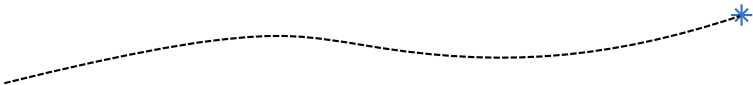

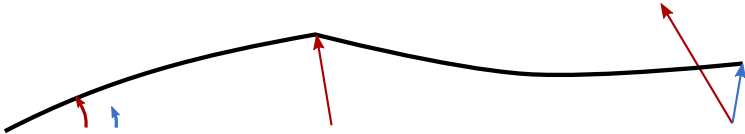

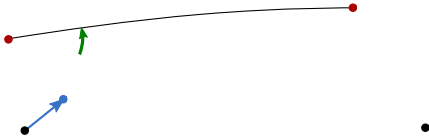

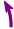

┐

┐

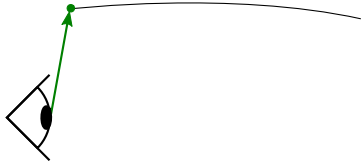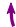



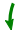

Supplement: Supplementary file 1 [file one_lens_3d_appendix.pdf]
